# Supplementary material for: Does the radio-active phase of XTE~J1810$-$197 recur following the same evolutionary pattern?
Source: arXiv:2601.07173 source file (2026-01-12)
Supplement: Supplementary file 1 [file Supplementary_Materials.pdf]

# Supplementary Materials

**Table S1.** Example of a Typical Timing Segment (MJD 59855–59861)

| Frequency<br>(MHz) | ToA<br>(MJD)          | ToA uncertainty<br>( $\mu$ s) |
|--------------------|-----------------------|-------------------------------|
| 2250               | 59855.336436978729003 | 613.752                       |
| 2250               | 59858.319353835974881 | 620.233                       |
| 2250               | 59859.324565768006580 | 542.481                       |
| 2250               | 59860.261065477606386 | 1712.736                      |
| 2250               | 59861.374573828591145 | 865.982                       |
| 8600               | 59855.335986393882443 | 846.831                       |
| 8600               | 59858.350789292825651 | 1195.079                      |
| 8600               | 59859.327194730493313 | 973.076                       |
| 8600               | 59861.390675767113174 | 1230.137                      |

**Table S2.** Timing solutions of XTE J1810–197 observations.

| Pepoch<br>(MJD) | Start<br>(MJD) | Finish<br>(MJD) | $\nu$<br>( $s^{-1}$ ) | $\dot{\nu}$<br>( $\times 10^{-13} s^{-2}$ ) | $N_{obs}$<br>- |
|-----------------|----------------|-----------------|-----------------------|---------------------------------------------|----------------|
| 59642           | 59636.83       | 59649.06        | 0.1804243489(9)       | -2.79(5)                                    | 6              |
| 59781           | 59775.65       | 59786.62        | 0.180421477(2)        | -2.5(1)                                     | 12             |
| 59804           | 59799.61       | 59809.65        | 0.180421031(2)        | -2.2(2)                                     | 9              |
| 59858           | 59855.33       | 59861.37        | 0.180419856(2)        | -2.5(2)                                     | 9              |
| 59954           | 59945.14       | 59963.07        | 0.180417824(1)        | -2.28(5)                                    | 6              |
| 60023           | 60014.87       | 60032.88        | 0.1804165798(8)       | -2.14(4)                                    | 7              |
| 60071           | 60068.82       | 60074.82        | 0.1804156793(7)       | -2.87(6)                                    | 7              |
| 60090           | 60085.69       | 60094.67        | 0.180415180(2)        | -2.3(3)                                     | 6              |
| 60120           | 60113.51       | 60127.71        | 0.180414451(3)        | -2.5(2)                                     | 11             |
| 60174           | 60171.48       | 60177.54        | 0.180413354(1)        | -2.0(2)                                     | 6              |
| 60196           | 60190.45       | 60202.49        | 0.180412970(1)        | -1.98(9)                                    | 7              |
| 60209           | 60207.36       | 60211.51        | 0.180412749(4)        | -2.0(8)                                     | 6              |
| 60219           | 60216.33       | 60223.40        | 0.180412614(1)        | -1.9(1)                                     | 6              |
| 60255           | 60240.31       | 60271.31        | 0.1804121221(7)       | -1.52(3)                                    | 6              |
| 60305           | 60301.28       | 60310.12        | 0.180411521(4)        | -1.4(3)                                     | 10             |
| 60310           | 60304.09       | 60317.01        | 0.180411459(5)        | -1.4(3)                                     | 10             |
| 60348           | 60338.08       | 60358.09        | 0.180411055(2)        | -1.17(8)                                    | 7              |
| 60363           | 60358.09       | 60367.96        | 0.180410898(6)        | -1.2(4)                                     | 9              |
| 60424           | 60418.71       | 60429.87        | 0.180410330(1)        | -0.9(1)                                     | 11             |
| 60501           | 60490.71       | 60512.46        | 0.1804096564(6)       | -1.02(2)                                    | 8              |
| 60529           | 60526.49       | 60531.61        | 0.180409404(3)        | -1.1(4)                                     | 4              |
| 60543           | 60539.55       | 60547.56        | 0.180409276(1)        | -1.06(2)                                    | 8              |

NOTE—Columns list the Period Epoch (Pepoch) of the timing solution, the start time and finish time of the observation span used for each fit (Start and Finish, respectively), the fitted spin frequency  $\nu$ , the first time derivative of its spin frequency  $\dot{\nu}$  and the total number of observations  $N_{obs}$  used in the solution.

**Table S3.** Parameters of XTE J1810–197 observations.

| MJD   | $T_{obs}$ | $S_{2.25}/S_{8.60}$ | $\alpha$  | $W_{10}$        | Shape | MJD   | $T_{obs}$ | $S_{2.25}/S_{8.60}$ | $\alpha$  | $W_{10}$        | Shape |
|-------|-----------|---------------------|-----------|-----------------|-------|-------|-----------|---------------------|-----------|-----------------|-------|
| –     | (min)     | (mJy)               | –         | (deg)           | –     | –     | (min)     | (mJy)               | –         | (deg)           | –     |
| 59636 | 200       | 2.72(5)/2.47(2)     | −0.072(2) | 36(3)/16.2(6)   | T/T   | 59643 | 60        | 2.66(8)/2.43(5)     | −0.07(3)  | 32(3)/16(1)     | T/T   |
| 59648 | 90        | 2.37(7)/2.32(3)     | −0.02(2)  | 33(3)/17(1)     | T/T   | 59775 | 60        | 7.46(8)/0.97(3)     | −1.52(3)  | 38(2)/16.8(9)   | T/T   |
| 59780 | 30        | 2.63(5)/0.68(4)     | −1.01(4)  | 31(7)/16(2)     | T/T   | 59781 | 30        | 2.24(4)/0.66(4)     | −0.91(6)  | 32(8)/16(1)     | T/T   |
| 59782 | 30        | 1.57(4)/0.65(5)     | −0.66(7)  | 33(0)/16(1)     | T/T   | 59784 | 30        | 2.34(2)/1.10(6)     | −0.56(6)  | 29(3)/15(3)     | T/T   |
| 59786 | 60        | 2.27(8)/1.53(3)     | −0.29(3)  | 32(4)/14.9(7)   | T/T   | 59799 | 230       | 1.70(4)/0.97(2)     | −0.42(3)  | 22(1)/14.8(6)   | T/T   |
| 59801 | 230       | 1.50(5)/0.66(2)     | −0.61(3)  | 30(2)/14.1(6)   | T/T   | 59806 | 60        | 1.94(8)/-           | -         | 38(4)/-         | T/-   |
| 59808 | 230       | 1.69(5)/0.80(2)     | −0.56(4)  | 32(2)/14.2(5)   | T/T   | 59809 | 20        | 2.46(4)/1.29(5)     | −0.48(4)  | 39(6)/14(1)     | T/T   |
| 59855 | 120       | 2.59(6)/2.74(2)     | 0.04(3)   | 23(1)/14.8(3)   | T/T   | 59858 | 120       | 3.53(7)/1.17(5)     | −0.82(2)  | 30(1)/15(1)     | D/D   |
| 59859 | 120       | 3.05(6)/1.40(2)     | −0.581(2) | 23.6(9)/14.4(9) | D/D   | 59860 | 15        | 3.73(9)/-           | -         | 28(4)/-         | D/-   |
| 59861 | 60        | 2.72(8)/0.61(3)     | −1.11(4)  | 30(2)/15.64(0)  | D/D   | 59913 | 30        | 1.50(6)/-           | -         | 30(6)/-         | D/-   |
| 59945 | 30        | 2.50(3)/0.49(2)     | −1.22(6)  | 28(4)/14(3)     | T/T   | 59955 | 25        | 2.20(6)/-           | -         | 30(6)/-         | T/-   |
| 59957 | 40        | 1.95(4)/-           | -         | 32(9)/-         | T/-   | 59963 | 40        | 2.27(1)/0.30(3)     | −1.51(5)  | 29(4)/15(3)     | T/T   |
| 59986 | 30        | 2.63(3)/-           | -         | 26(3)/-         | T/-   | 60014 | 30        | 1.54(3)/-           | -         | 31(7)/-         | T/-   |
| 60025 | 40        | 3.50(1)/1.82(2)     | −0.49(3)  | 30(9)/15.9(3)   | Q/Q   | 60028 | 30        | 2.05(4)/0.97(2)     | −0.558(2) | 31(4)/14.3(7)   | Q/Q   |
| 60032 | 30        | 2.40(2)/0.98(5)     | −0.67(3)  | 28(2)/14(1)     | Q/Q   | 60036 | 150       | 2.38(6)/2.74(2)     | 0.11(2)   | 29(1)/15.4(2)   | Q/Q   |
| 60068 | 120       | 2.81(6)/2.59(2)     | −0.06(3)  | 32(4)/14.1(6)   | Q/Q   | 60070 | 30        | 1.59(4)/1.54(6)     | −0.02(4)  | 28(7)/15(6)     | Q/Q   |
| 60072 | 60        | 2.75(8)/-           | -         | 30(1)/-         | T/-   | 60074 | 30        | 3.63(5)/3.68(6)     | 0.01(6)   | 34(6)/15(1)     | Q/Q   |
| 60081 | 120       | 4.19(6)/2.48(2)     | −0.39(7)  | 30(2)/14.3(5)   | Q/Q   | 60083 | 120       | 2.35(7)/-           | -         | 31(5)/-         | Q/-   |
| 60085 | 30        | 2.04(4)/0.95(5)     | −1.36(6)  | 32(6)/16(2)     | T/T   | 60090 | 120       | 1.53(7)/0.46(5)     | −0.02(3)  | 30(6)/15(3)     | T/T   |
| 60094 | 30        | 3.67(5)/1.97(4)     | −0.46(3)  | 31(4)/15(4)     | T/T   | 60102 | 40        | 2.71(0)/-           | -         | 28(2)/-         | D/-   |
| 60113 | 30        | 0.97(2)/-           | -         | 31(8)/-         | D/-   | 60114 | 20        | 1.2(2)/-            | -         | 35(8)/-         | D/-   |
| 60116 | 30        | 2.48(3)/0.98(4)     | −0.69(3)  | 36(4)/16(1)     | D/D   | 60117 | 30        | 2.01(3)/1.47(4)     | −0.23(4)  | 36(5)/16(5)     | D/D   |
| 60118 | 60        | 2.50(0)/-           | -         | 32(3)/-         | D/-   | 60125 | 120       | 2.54(7)/0.67(3)     | −0.99(4)  | 26(1)/16(1)     | D/D   |
| 60127 | 60        | 1.85(9)/1.07(3)     | −0.41(3)  | 33(3)/16(1)     | D/D   | 60171 | 60        | 2.33(9)/1.86(3)     | −0.17(2)  | 31(2)/13.7(6)   | D/D   |
| 60175 | 30        | 1.20(3)/1.63(4)     | 0.228(2)  | 34(6)/16(1)     | D/D   | 60177 | 60        | 1.60(0)/0.41(4)     | −1.02(4)  | 36(5)/15(3)     | D/D   |
| 60190 | 60        | 1.22(8)/0.30(3)     | −1.05(6)  | 35(4)/16(4)     | D/D   | 60195 | 120       | 1.33(6)/1.91(2)     | 0.27(5)   | 29(3)/14.1(4)   | D/D   |
| 60200 | 30        | 1.53(3)/-           | -         | 30(6)/-         | D/-   | 60202 | 30        | 1.26(3)/0.58(4)     | −0.58(3)  | 28(7)/15(2)     | D/D   |
| 60207 | 40        | 0.89(1)/1.39(6)     | 0.333(2)  | 29(7)/15(2)     | D/D   | 60209 | 120       | 0.53(6)/0.14(4)     | −0.99(3)  | 31(6)/15(5)     | D/D   |
| 60211 | 30        | 0.83(2)/1.13(7)     | 0.23(2)   | 26(7)/14(2)     | D/D   | 60216 | 120       | 1.01(6)/0.98(2)     | −0.02(3)  | 26(4)/14.8(4)   | D/D   |
| 60218 | 120       | 0.51(6)/0.57(2)     | 0.08(4)   | 29(5)/14(1)     | D/D   | 60223 | 138       | 1.03(7)/1.77(3)     | 0.40(6)   | 30(4)/14.8(7)   | D/D   |
| 60240 | 30        | 1.23(4)/0.49(5)     | −0.69(7)  | 30(6)/15(3)     | D/D   | 60258 | 30        | 1.73(5)/0.48(5)     | −0.96(6)  | 32(5)/16(3)     | D/D   |
| 60271 | 30        | 1.31(3)/0.78(4)     | −0.39(3)  | 24(6)/17(2)     | D/D   | 60301 | 30        | 0.7(2)/0.58(4)      | −0.17(3)  | 27(2)/15(3)     | D/D   |
| 60303 | 60        | 1.32(1)/0.47(3)     | −0.77(3)  | 29(5)/16(3)     | D/D   | 60304 | 30        | 1.42(8)/0.98(6)     | −0.28(4)  | 31(1)/15(1)     | D/D   |
| 60308 | 30        | 1.04(8)/0.47(8)     | −0.83(4)  | 23(5)/15(4)     | D/D   | 60310 | 180       | 0.87(6)/0.47(2)     | −0.46(3)  | 22(2)/15(1)     | D/D   |
| 60315 | 60        | 0.89(0)/1.23(3)     | 0.24(2)   | 22(3)/10.9(4)   | D/D   | 60316 | 60        | 1.25(2)/0.73(3)     | −0.401(2) | 14(3)/12(2)     | D/D   |
| 60338 | 60        | 1.01(9)/0.55(4)     | −0.45(4)  | 14(2)/14(3)     | D/D   | 60345 | 60        | 0.59(0)/-           | -         | 18(6)/-         | D/-   |
| 60347 | 30        | 1.04(3)/0.34(5)     | −0.83(6)  | 20(7)/13(3)     | D/D   | 60358 | 30        | 2.21(3)/0.95(8)     | −0.63(5)  | 18(1)/13(1)     | D/D   |
| 60360 | 60        | 0.60(9)/-           | -         | 14(4)/-         | D/-   | 60362 | 30        | 0.26(7)/0.50(5)     | 0.49(3)   | 12(8)/13(1)     | D/D   |
| 60363 | 60        | 0.60(9)/0.58(4)     | −0.025(2) | 19(5)/13(1)     | D/D   | 60367 | 30        | 0.14(4)/0.56(5)     | 1.03(3)   | 15(5)/12(7)     | D/D   |
| 60418 | 30        | 2.06(3)/0.97(5)     | −0.56(2)  | 13(1)/12(1)     | D/D   | 60420 | 60        | 1.83(9)/1.22(3)     | −0.30(3)  | 12.3(7)/12.0(6) | D/D   |
| 60426 | 30        | 1.11(3)/0.81(4)     | −0.23(4)  | 13(1)/11.5(7)   | D/D   | 60427 | 60        | 1.63(9)/-           | -         | 12.7(8)/-       | D/-   |
| 60428 | 60        | 2.02(9)/1.79(3)     | −0.09(6)  | 13.0(6)/11.6(3) | D/D   | 60429 | 60        | 2.14(9)/2.04(3)     | −0.04(7)  | 12.7(5)/11.6(4) | D/D   |
| 60490 | 60        | 0.32(0)/0.84(3)     | 0.72(6)   | 12(6)/11.2(7)   | D/D   | 60491 | 60        | 0.65(9)/0.78(5)     | 0.14(3)   | 12(4)/11(1)     | D/D   |
| 60500 | 30        | 0.49(4)/0.61(5)     | 0.16(3)   | 12(2)/10.9(6)   | D/D   | 60503 | 30        | 1.19(4)/1.40(5)     | 0.12(3)   | 13(1)/10.5(4)   | D/D   |
| 60511 | 30        | 2.50(3)/1.30(4)     | −0.49(4)  | 12.7(7)/12.0(7) | D/D   | 60512 | 30        | 0.81(5)/0.72(4)     | −0.09(4)  | 12(3)/11.6(5)   | D/D   |
| 60526 | 30        | 2.47(3)/2.33(7)     | −0.04(3)  | 12(1)/10.3(7)   | D/D   | 60527 | 30        | 1.57(2)/1.12(5)     | −0.25(2)  | 11.6(9)/10.2(4) | D/D   |
| 60528 | 30        | 2.03(4)/1.01(5)     | −0.521(2) | 12(1)/11(1)     | D/D   | 60531 | 30        | 2.63(3)/1.70(4)     | −0.33(4)  | 12.3(8)/10.9(5) | D/D   |
| 60539 | 30        | 4.37(3)/1.41(4)     | −0.84(6)  | 12.7(6)/11.2(4) | D/D   | 60541 | 30        | 3.76(3)/1.40(4)     | −0.74(5)  | 11.2(5)/10.9(5) | D/D   |
| 60545 | 30        | 3.8(2)/3.55(5)      | −0.05(3)  | 12(2)/10.8(3)   | D/D   | 60547 | 30        | 6.34(3)/4.26(4)     | −0.30(4)  | 12.3(5)/10.3(3) | D/D   |
| 60553 | 30        | 1.17(4)/-           | -         | 12(3)/-         | D/-   | 60583 | 30        | 1.60(2)/0.11(5)     | −2.01(6)  | 12(1)/10(8)     | D/D   |
| 60595 | 30        | 0.3↓/0.1↓           | -         | -/-             | -/-   | 60612 | 30        | 0.3↓/0.1↓           | -         | -/-             | -/-   |

NOTE—Columns list the start time of each observation (MJD), the length of observation  $T_{obs}$  in minutes, the measured mean flux densities at 2.25 and 8.60 GHz ( $S_{2.25}/S_{8.60}$ ) in mJy (or upper limits for non-detections), the spectral index  $\alpha$ , the full width at 10% maximum  $W_{10}$  of the combined P1/P2 emission region (in degrees), and the morphological classification of the integrated pulse profile: D (double-peaked), T (triple-peaked), or Q (quadruple-peaked). For the final two non-detection epochs (MJD 60595 and 60612),  $3\sigma$  upper limits on flux density are reported assuming the same profile shape as the last high-S/N detection.

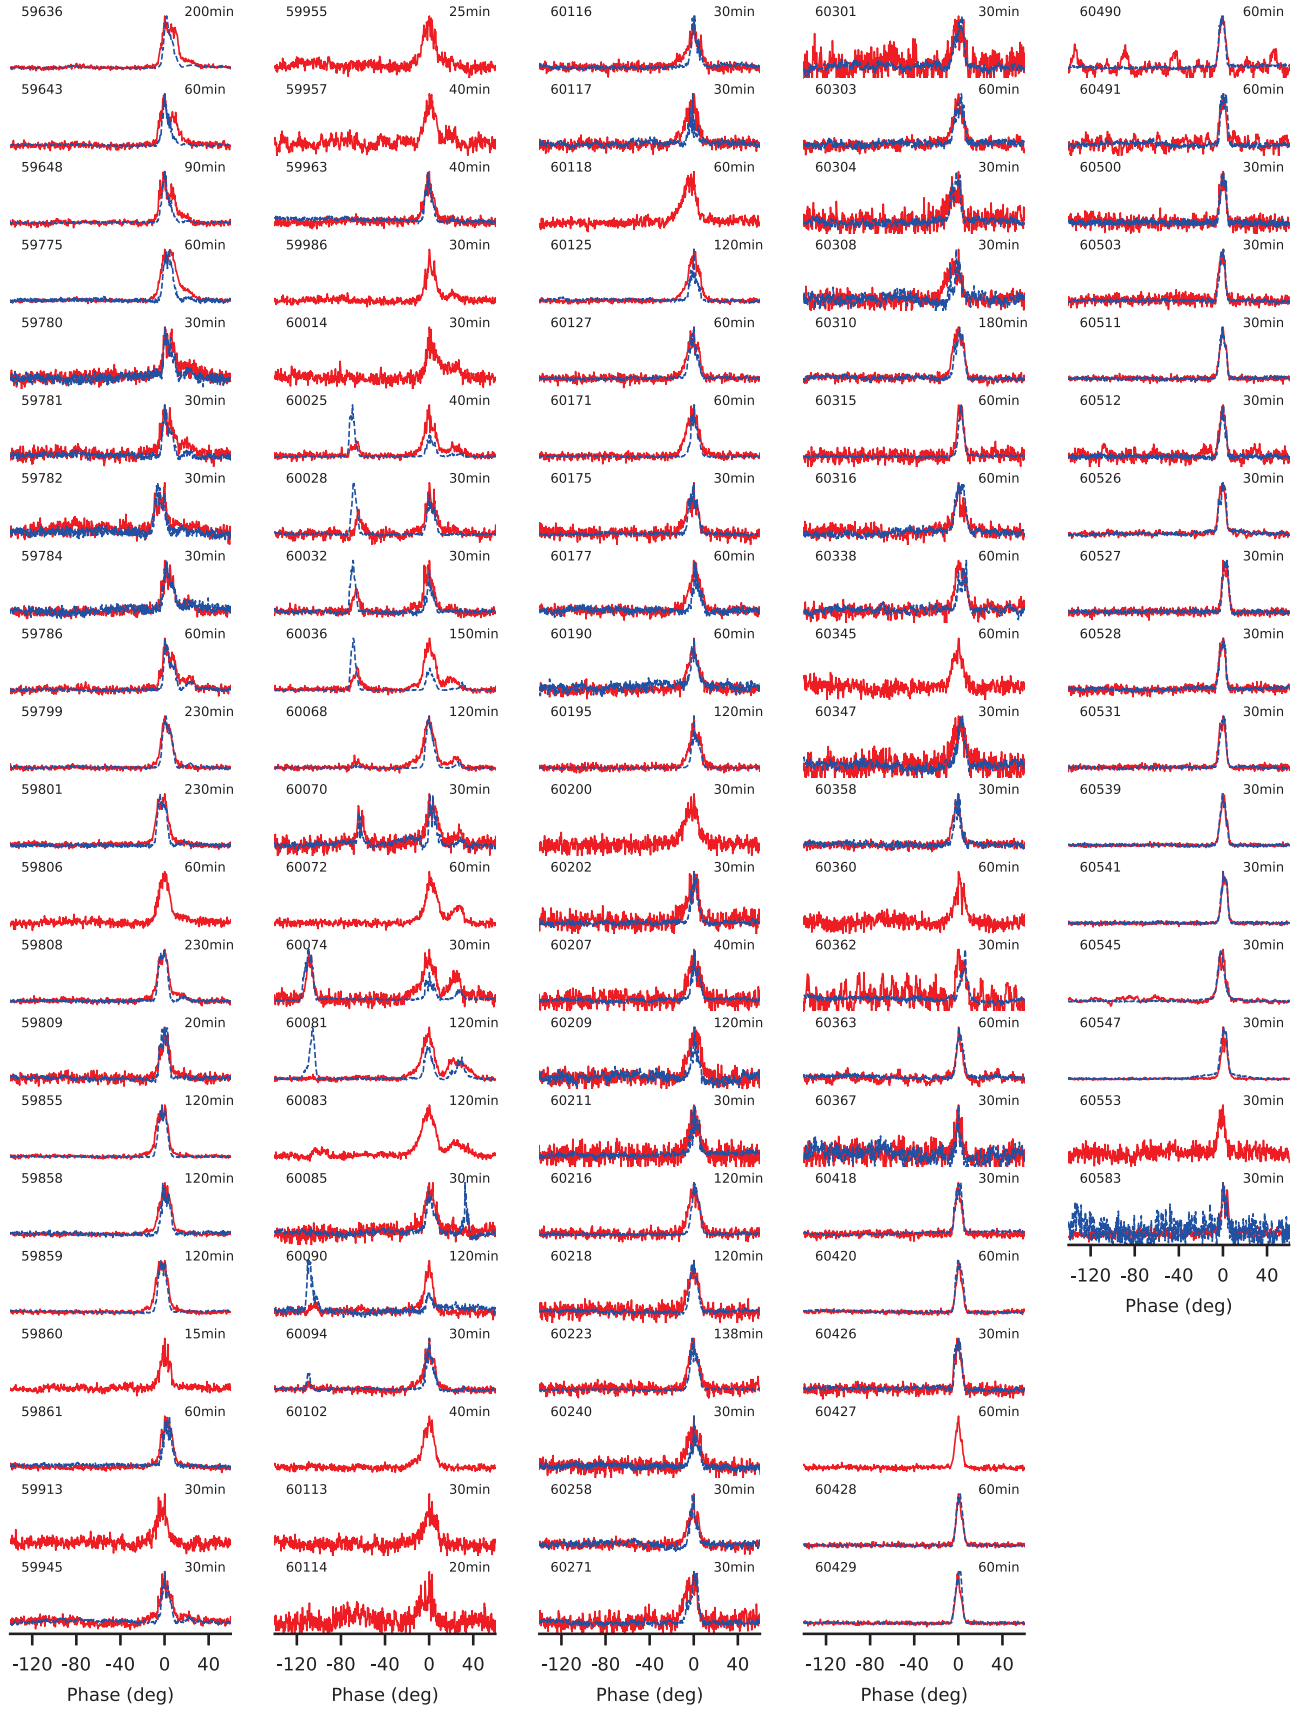

**Figure S1.** Normalized integrated profiles of magnetar XTE J1810-197 during MJD 59636-60583. Profiles at 2.25 GHz and 8.60 GHz are represented by red and dotted blue line, respectively. Observational epoch (MJD) and integration time are annotated in the upper-left and upper-right corner of each panel.
